# Supplementary material for: Beyond the Hype: A Real-World Evaluation of the Impact and Cost of Machine Learning-Based Malware Detection
Source: arXiv:2012.09214 source file (2022-08-17)
Supplement: Supplementary file 1 [file 99-appendix.tex]

\section*{Appendix}
\appendix
\begin{figure}[!h]
    \centering
    \includegraphics[width=\textwidth]{fig/ncr-network-diagram-sanitized.png}
    \caption{\hl{Network Diagram}}
    \label{fig:network-diagram}
\end{figure}
